# Supplementary material for: On Mitigating Code LLM Hallucinations with API Documentation
Source: arXiv:2407.09726 source file (2024-07-13)
Supplement: Supplementary file 1 [file low-freq-deep-dive.tex]

\begin{table*}
\centering
\resizebox{\textwidth}{!}{%

    \begin{tabular}{c|cc|ccc}
    \hline
    \hline
    \multirow{2}{*}{\textbf{Model}} & \multirow{2}{*}{\textbf{Valid (\%)}} & \multirow{2}{*}{\textbf{Invalid (\%)}} & \multicolumn{3}{c}{\textbf{Invalid API Inv.}} \\
    & & & \textit{UIE} & \textit{IUC} & \textit{UNE} \\
    \hline
    Google CodeGemma-7B                                & $12.36$ & $87.64$ & $10.68$ & $35.47$ & $53.85$ \\
    StarCoder2-15B                                     & $24.72$ & $75.28$ & $10.95$ & $33.33$ & $55.72$ \\
    IBM Granite-Code-20B                               & $32.21$ & $67.79$ & $17.13$ & $23.76$ & $59.12$ \\
    DeepSeekCoder-33B                                  & $34.83$ & $65.17$ & $15.52$ & $31.03$ & $53.45$ \\
    GPT-4o                                             & $38.58$ & $61.42$ & $13.41$ & $33.54$ & $53.05$ \\
    \hline
    \hline

    \end{tabular}
}%
\caption{\textbf{Results on \bench.}}
\label{tab:appendix-low-freq-deep-dive}
\end{table*}
